# Supplementary material for: Revitalizing Optimization for 3D Human Pose and Shape Estimation: A Sparse Constrained Formulation
Source: arXiv:2105.13965 source file (2021-10-04)
Supplement: Supplementary file 2 [file notation.tex]

\def\0{\boldsymbol{0}}

\def\se3{\mathfrak{se}(3)}

\long\def\answer#1{}

\long\def\comment#1{}

\theoremstyle{definition}

\def\int{\mathrm{int}}

\crefname{prop}{Proposition}{Propositions}
\crefname{problem}{Problem}{Problems}

\theoremstyle{remark}
\newtheorem*{remark*}{{Remark}}

\newcolumntype{P}[1]{>{\centering\arraybackslash}p{#1}}

\newcolumntype{P}[1]{>{\centering\arraybackslash}p{#1}}
\newcolumntype{M}[1]{>{\centering\arraybackslash}m{#1}}
